# Supplementary material for: Quantum Criticality from Spectral Collapse in the Two-Photon Rabi Model
Source: arXiv:2604.23164 source file (2026-09-16)
Supplement: Supplementary file 1 [file Supplementary_Material.tex]

\documentclass[prl,print,preprintnumbers,longbibliography]{revtex4-2}

\usepackage{amsfonts}
\usepackage{amssymb}
\usepackage{amsmath}
\usepackage{graphicx}
\usepackage{bm}
\usepackage{color}
\usepackage{braket}
\usepackage[colorlinks=true, allcolors=blue, breaklinks]{hyperref}
\usepackage{float}

\usepackage[utf8]{inputenc}

\raggedbottom

\begin{document}
	
	\title{Quantum criticality from spectral collapse in the two-photon Rabi model\\
		-Supplementary Material-
	}
	
	\author{Jiong Li$^{1}$}
	\author{Jun-ling Wang$^{2}$}
	\author{Qing-Hu Chen$^{2,1,3,}$}
	\email{qhchen@zju.edu.cn}
	\author{Hai-Qing Lin$^{1,}$}
	\email{hqlin@zju.edu.cn}
	
	\affiliation{
		$^1$ Institute for Advanced Study in Physics and School of Physics, Zhejiang University, Hangzhou 310027, China \\
		$^2$ Zhejiang Key Laboratory of Micro-Nano Quantum Chips and Quantum Control, School of Physics,
		Zhejiang University, Hangzhou, Zhejiang 310027, China. \\
		$^3$ Collaborative Innovation Center of Advanced Microstructures, Nanjing University, Nanjing 210093, China.
	}
	\date{\today}
	
	\maketitle
	
	\section{Asymptotic Exactness of the Adiabatic Approximation}
	
	In this section, we show that the adiabatic approximation (AA) becomes asymptotically exact in the vicinity of the critical line and provides a controlled low-energy description emergent of the soft-mode physics discussed in the main text. Our strategy is to derive a systematic hierarchy of corrections and to show that all off-diagonal processes are parametrically suppressed near criticality.
	
	The Hamiltonian of the anisotropic two-photon quantum Rabi model (tpQRM) is 
	\begin{equation}
		H = - \frac{\Delta}{2} \sigma_x+\omega a^\dagger a + g \frac{1+r}{2} \sigma_{z} \left( a^2 + a^{\dagger 2} \right)  + g \frac{1-r}{2} i \sigma_y \left( a^2 - a^{\dagger 2} \right).
		\label{H_0}
	\end{equation}
	Owing to the conserved symmetry $\Pi = -\sigma_x \exp \left(i \frac{\pi}{2} a^\dagger a\right)$, the eigenstate can be written as
	\begin{equation}
		\ket{\Phi} =
		\begin{bmatrix}
			\sum_{n=0}^{\infty} c_n S(-\theta) \ket{2n} \\
			\mp \sum_{n=0}^{\infty} (-1)^n c_n S(\theta) \ket{2n}
		\end{bmatrix}.
		\label{phi}
	\end{equation}
	where the $\mp$ sign corresponds to parity eigenvalues $\pm 1$.
	
	Introducing the squeezing parameter
	\begin{equation}
		\theta = \frac{1}{4}\ln \frac{1 + g/g_c}{1 - g/g_c}, \quad g_c = \frac{1}{1+r},
	\end{equation}
	the Hamiltonian is transformed into harmonic blocks 
	\begin{equation}
		S(\theta) H_{11} S(-\theta) = S(-\theta) H_{22} S(\theta) = \left( a^\dagger a + \frac{1}{2} \right) \beta - \frac{1}{2},
	\end{equation}
	with an effective frequency $\beta = \sqrt{1-g^2/g_c^2}$. The problem is thus reduced to coupled quasiparticle sectors with a vanishing frequency $\beta \to 0$ at the critical line.
	
	Projecting the Schr\"odinger equation $H \ket{\Phi} = E \ket{\Phi}$ onto $\bra{2m} S(\theta)$ yields an infinite set of coupled equations,
	\begin{equation}
		0 = c_m \left[\left( 2m+\frac{1}{2} \right) \beta - \frac{1}{2} - E \right] \pm \sum_{n=0}^{\infty} c_n M_{mn}(\beta),
		\label{inf_matrix}
	\end{equation}
	which serves as the starting point of the AA. The matrix elements $M_{mn}(\beta)$ encode the coupling between different photonic manifolds 
	\begin{equation}
		M_{mn}(\beta) = \bra{2m} S(-\theta) \left[ -\frac{\Delta}{2} \sigma_x + g \frac{1-r}{2} i \sigma_y \left( a^2 - a^{\dagger 2} \right) \right] \ket{2n}
	\end{equation}
	and can be expressed in terms of associated Legendre polynomials $P_l^k(x)$ as
	\begin{equation}
		M_{mn}(\beta) = (-1)^m \sqrt{\beta} \sqrt{\frac{(2n)!}{(2m)!}} \bigg[ \frac{\Delta}{2} P_{m+n}^{m-n} (\beta) - g \frac{1-r}{2} \left( P_{m+n-1}^{m-n+1} (\beta) - (2n+1)(2n+2) P_{m+n+1}^{m-n-1} (\beta) \right) \bigg],
	\end{equation}
	through
	\begin{equation}
		\bra{2m} S(-2\theta) \ket{2n} = (-1)^{m-n} \sqrt{\beta} \sqrt{\frac{\left( 2n \right)!}{\left( 2m \right)!}} P_{m+n}^{m-n} (\beta), \quad \bra{2m} S(2\theta) \ket{2n} = \sqrt{\beta} \sqrt{\frac{ \left( 2n \right)! }{\left( 2m \right)!}} P_{m+n}^{m-n} (\beta).
	\end{equation}
	
	Within the AA, neglecting off-diagonal couplings between different photonic manifolds yields eigenstates
	\begin{equation}
		\ket{\psi_{n,\pm}^{(\rm AA)}} = \frac{1}{\sqrt{2}} \begin{bmatrix}
			S(-\theta) \ket{2n} \\
			\mp (-1)^n S(\theta) \ket{2n}
		\end{bmatrix},
	\end{equation}
	with eigenenergies
	\begin{equation}
		E_{n,\pm}^{\rm (AA)} = \left( 2n + \frac{1}{2} \right) \beta - \frac{1}{2} \pm M_{nn} (\beta) = \left( 2n + \frac{1}{2} \right) \beta - \frac{1}{2} \pm (-1)^n \sqrt{\beta} \left[ \frac{\Delta}{2} P_{2n}^{0} (\beta) - g \frac{1-r}{2} \left( P_{2n-1}^{1} (\beta) + P_{2n+1}^{1} (\beta) \right) \right].
	\end{equation}
	
	For $\beta \ll 1$, the associated Legendre functions admit the expansion
	\begin{equation}
		P_\ell^k (\beta) = \left[1 - (\ell+k+1) \frac{\ell-k}{2} \beta^2 + \mathcal{O} (\beta^4) \right] \frac{(\ell+k-1) !! (-1)^\frac{\ell-k}{2}}{\left( \ell-k \right)!!} (1-\beta^2)^\frac{k}{2},
	\end{equation}
	which yields
	\begin{equation}
		M_{mn}(\beta) = (-1)^{m+n} \frac{\sqrt{\beta}}{2} K_{mn}(\beta) \left[ \delta + \alpha_{mn} \beta^2 + \mathcal{O} (\beta^4) \right],
	\end{equation}
	with
	\begin{eqnarray}
		K_{mn}(\beta) &=& \sqrt{\frac{(2m-1)!! (2n-1)!!}{(2m)!! (2n)!!}} \left( 1-\beta^2 \right)^\frac{\vert m-n \vert}{2}, \nonumber \\
		\alpha_{mn} &=& (2m+1) \left( (5n+1) \Delta_c - n \Delta \right) - 2n \Delta_c.
		\nonumber \\
		\delta &=& \Delta - \Delta_c. 
	\end{eqnarray}	
	The prefactor $\sqrt{\beta}$ sets the overall scaling, while $K_{mn}(\beta)$ suppresses off-diagonal matrix elements. 
	
	\begin{figure}[tbp]
		\includegraphics[width=1.0\linewidth]{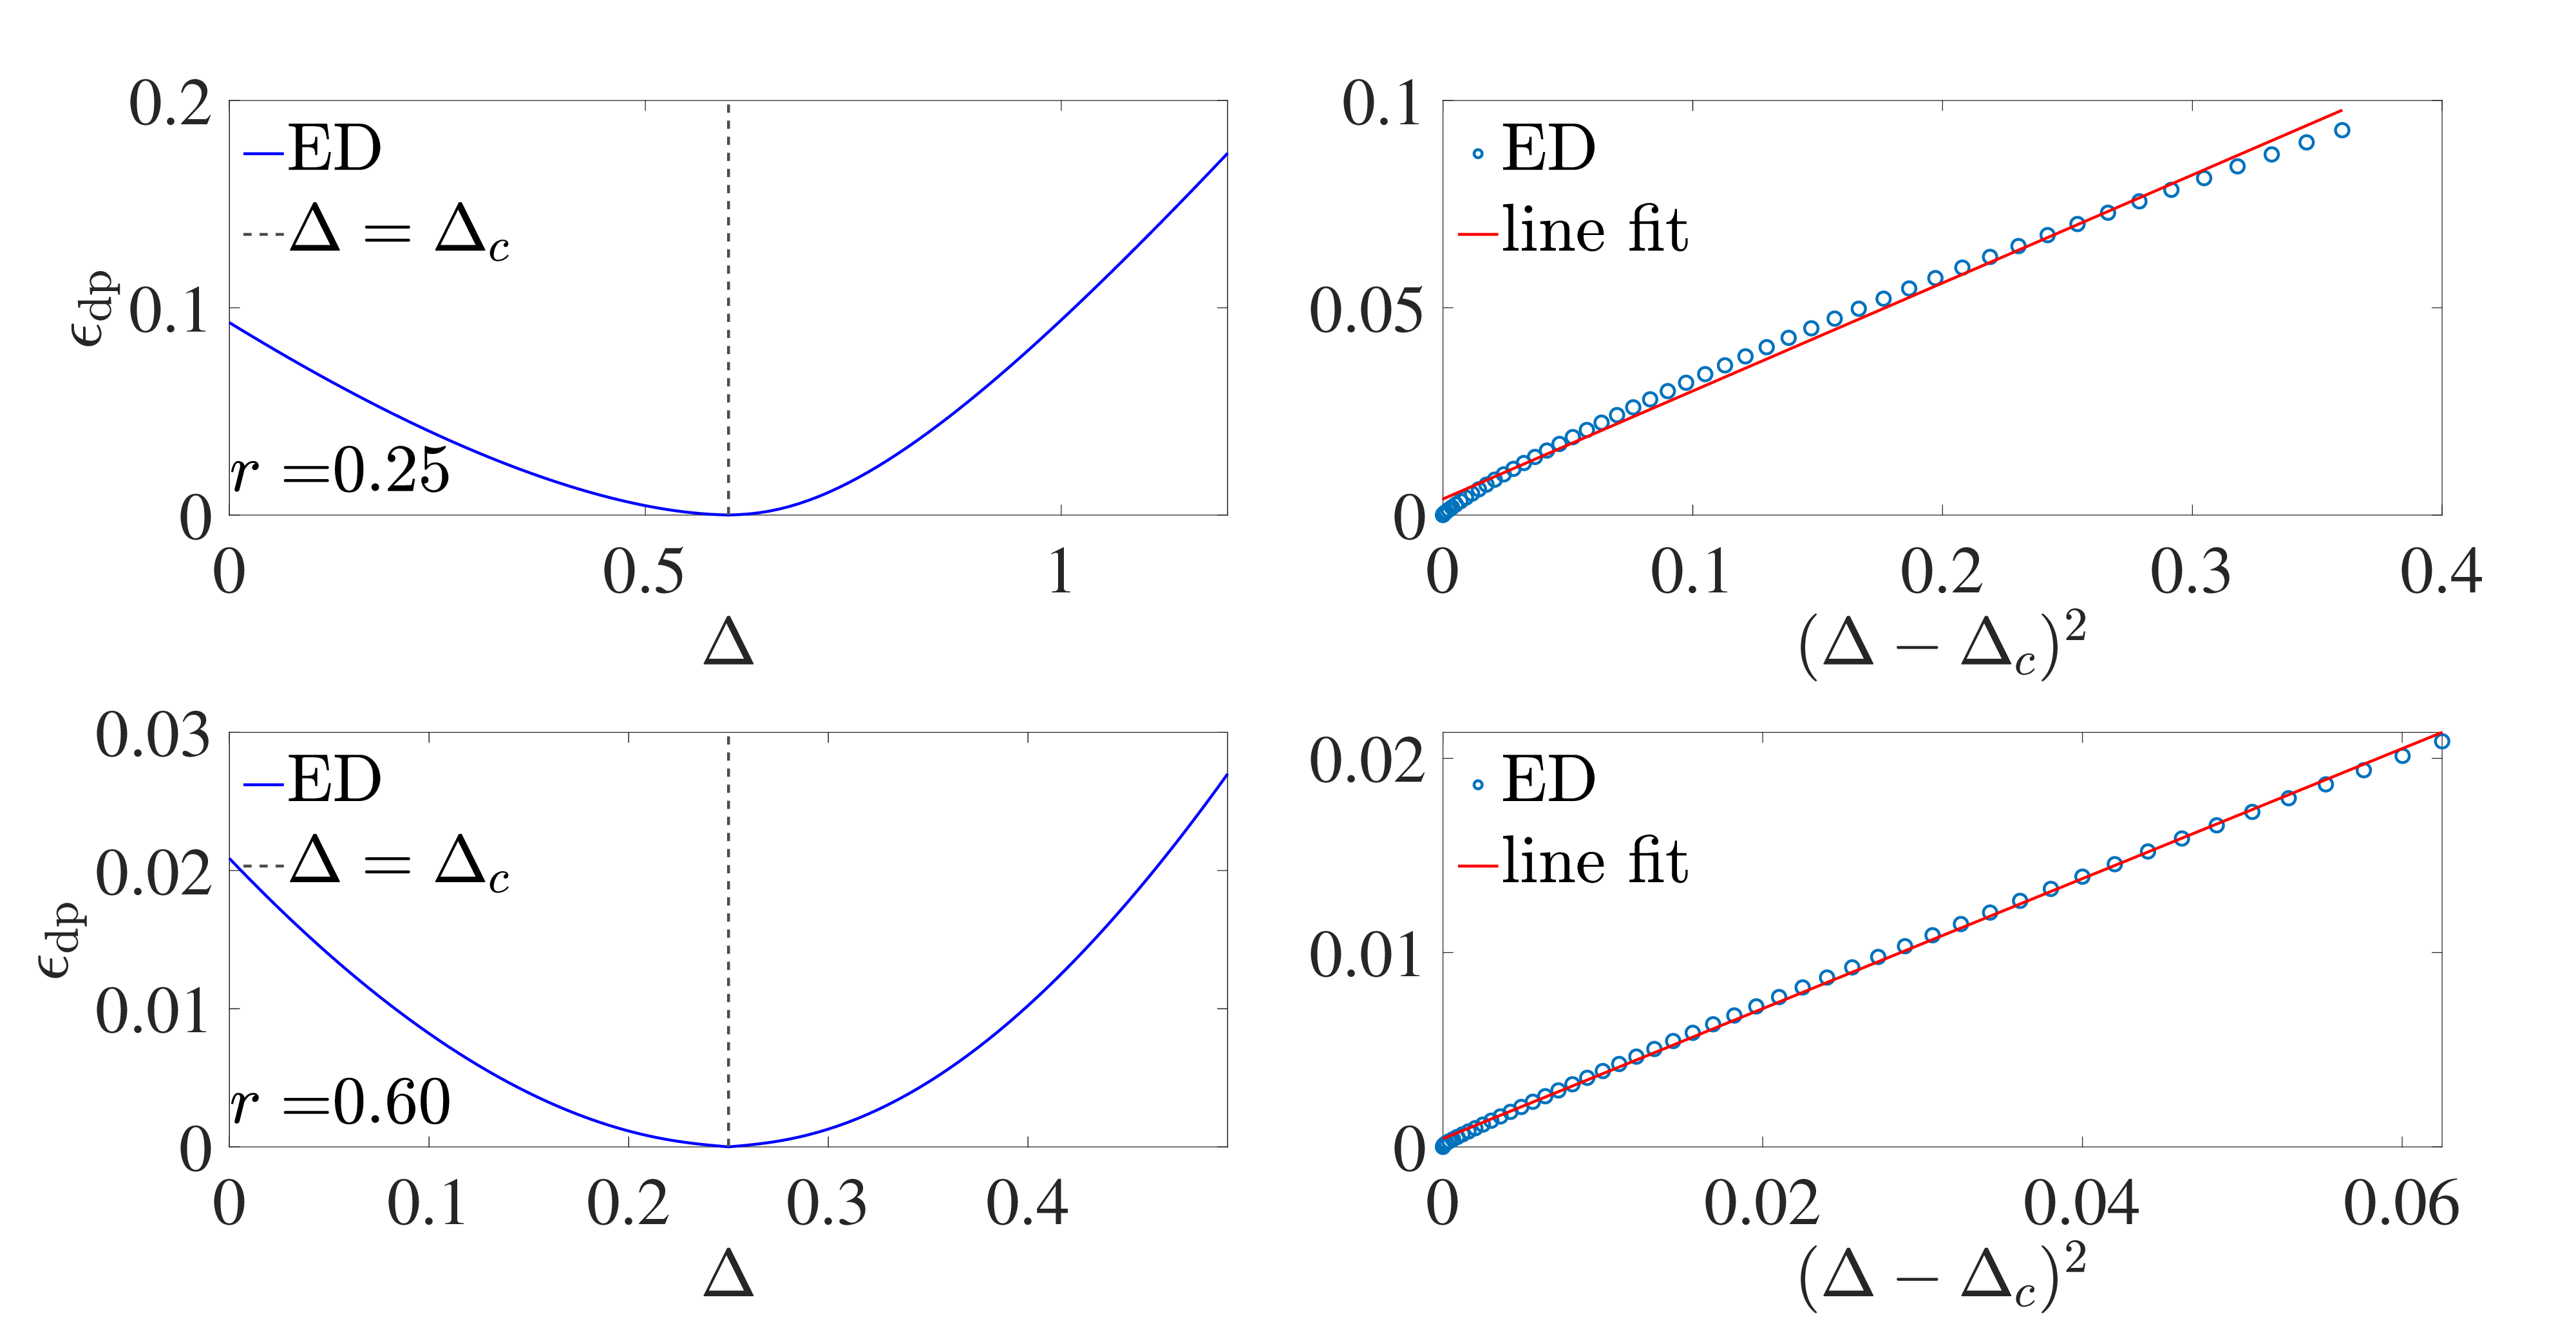}
		\caption{Left: Energy gap $\epsilon_{\rm dp}$ at $g=g_{c}$ as a function of $\Delta$ obtained by exact diagonalization for $r=0.25$ (upper panels) and $r=0.60$ (lower panels). The black dashed line marks the critical value $\Delta_c$. Right: Same data replotted as a function of $(\Delta - \Delta_c)^2$ for $\Delta < \Delta_c$ (open circles). The red line shows a linear fit.}
		\label{fig_energygap}
	\end{figure}
	
	This yields the AA spectrum near the collapse point [Eq.~(5) of the main text],
	\begin{equation}
		E_{n,\pm}^{(\rm AA)} \simeq \left(2n + \frac{1}{2} \right) \beta - \frac{1}{2} \pm \frac{\sqrt{\beta}}{2} \frac{(2n-1)!!}{(2n)!!} \left( \delta + \alpha_{nn} \beta^{2} \right),
	\end{equation}
	from which the hierarchy of excitation gaps follows [Eqs.~(6) and (7) of the main text], 
	\begin{eqnarray}
		\epsilon_{\rm sp} = \left| E_{n+1,\pm} - E_{n,\pm} \right| &\propto& \beta \propto |g - g_c|^{z\nu}, \quad z\nu = \frac{1}{2}, \nonumber\\
		\epsilon_{\rm dp} = \left| E_{n,+} - E_{n,-} \right| &\propto& \beta^{5/2} \propto |g - g_c|^{\mu}, \quad \mu = \frac{5}{4}.
	\end{eqnarray}
	The gap within the same parity $\epsilon_{\rm sp}$ defines the soft mode responsible for the critical behavior, whereas the gap between different parities $\epsilon_{\rm dp}$ arises from symmetry-induced level splitting and does not correspond to a critical excitation. This separation of energy scales is the origin of the universal scaling structure.
	
	To assess the validity of the AA, we include off-diagonal corrections within perturbation theory. The corrections to the eigenstates scale as
	\begin{equation}
		\ket{\psi_{n,\pm}^{(\rm off)}} \simeq \sum_{m \neq n} \frac{M_{mn}(\beta) \ket{\psi_{m,\pm}^{(\rm AA)}}}{E_m^{(\rm AA)} - E_n^{(\rm AA)}}  \sim \sum_{m \neq n} (-1)^{m+n} \frac{ \sqrt{\beta} K_{mn}(\beta) \left( \delta + \alpha_{mn} \beta^2 \right)}{4(m-n) \beta} \ket{\psi_{m,\pm}^{(\rm AA)}} \sim
		\begin{cases}
			\mathcal{O}(\beta^{-1/2}), & \delta \neq 0, \\
			\mathcal{O}(\beta^{3/2}), & \delta = 0,
		\end{cases}
	\end{equation}
	indicating strong mixing away from criticality but vanishing corrections exactly at $\delta=0$. The corresponding energy corrections scale as
	\begin{equation}
		E_{n,\pm}^{(\rm off)} \simeq \sum_{m \neq n} \frac{\vert M_{mn} (\beta)\vert^2} { E_{m}^{(\rm AA)} - E_{n}^{(\rm AA)}} 
		\sim \sum_{m \neq n} \frac{ \beta K_{mn}^2 (\beta) \left( \delta + \alpha_{mn} \beta^2 \right)^2}{8(m-n) \beta} \sim
		\begin{cases}
			\mathcal{O}(\delta^2), & \delta \neq 0, \\
			\mathcal{O}(\beta^4), & \delta = 0,
		\end{cases}
	\end{equation}
	which remains finite for $\delta \neq 0$, but is of $\mathcal{O}(\beta^4)$ at $\delta = 0$ and are therefore subleading compared to the AA spectrum. 
	
	These results show that off-diagonal processes are parametrically suppressed near the critical line, and do not modify the scaling of excitation gaps. The AA thus becomes asymptotically exact for $\Delta=\Delta_c$ and provides an effective description of the soft-mode sector.    
	
	Furthermore, the gap opening $\epsilon_{\rm dp} \propto \delta^2$ for $\Delta \neq \Delta_c$ is consistent with the numerical results in Fig.~\ref{fig_energygap}, providing quantitative support for the analytical scaling.
	
	Taken together, this analysis establishes a controlled hierarchy of energy scales and demonstrates that the universal critical behavior is entirely governed by the single soft mode. Consequently, the critical exponents $z\nu = 1/2$ and $\mu = 5/4$ are robust throughout the anisotropic regime, providing a microscopic foundation for the universal scaling structure discussed in the main text.
	
	\section{Spectral Collapse in the Isotropic tpQRM}
	
	In this section, we provide a microscopic interpretation of spectral collapse in the isotropic tpQRM ($r=1$) and clarify its relation to the soft-mode physics discussed in the main text. Our strategy is to reformulate the model in phase space and analyze the structure of the low-energy spectrum across the collapse point.
	
	In the isotropic limit, the Hamiltonian reduces to
	\begin{equation}
		H_{\rm tp} = - \frac{\Delta}{2} \sigma_x+\omega a^\dagger a + g \sigma_{z} \left( a^2 + a^{\dagger 2} \right).
	\end{equation}
	Introducing the canonical position and momentum operators, $x = a + a^\dagger$ and $p = i(a^\dagger - a)$, the Hamiltonian can be rewritten as
	\begin{equation}
		H_{\rm tp} = \frac{1}{2} \begin{bmatrix}
			\left( \frac{1}{2} + g \right) x^2 + \left( \frac{1}{2} - g \right) p^2 - 1 & -\Delta \\
			-\Delta & \left( \frac{1}{2} - g \right) x^2 + \left( \frac{1}{2} + g \right) p^2 - 1
		\end{bmatrix}.
	\end{equation}
	Note that here $p=-2i \partial_x$. This representation makes explicit that the system consists of two coupled quadratic modes with an effective frequency $\omega_{\rm eff} = \sqrt{1 - 4g^2}$, which vanishes at $g_c = 1/2$. The collapse point is therefore characterized by the disappearance of harmonic confinement along a canonical direction.
	
	In the Rabi-Stark model, at the collapse point, the Hamiltonian is significantly reduced and can be solved analytically~\cite{xie_quantum_2019}. Similarly, for the tpQRM, the Hamiltonian at the collapse point $g = g_c$ can simplified as
	\begin{equation}
		H_{\rm c} = \frac{1}{2} \begin{bmatrix}
			x^2 - 1 & -\Delta \\
			-\Delta &  p^2 - 1
		\end{bmatrix},
	\end{equation}
	where one quadrature is no longer confined, reflecting the flattening of the effective potential along a canonical direction. This provides a direct phase-space picture of spectral collapse as the loss of confinement.
	
	To analyze the resulting spectrum, we consider the Schr\"odinger equation for wavefunction $\varphi = [\varphi_1 \, \varphi_2]^{\rm T}$:
	\begin{equation}
		\frac{1}{2} \left( x^2 \varphi_1 - \Delta \varphi_2 \right) = \left( E+\frac{1}{2} \right) \varphi_1, \quad
		\frac{1}{2} \left( -\Delta \varphi_1 - 4 \partial_x^2 \varphi_2 \right) = \left( E+\frac{1}{2} \right) \varphi_2.
	\end{equation}	
	For $r=1$, the corresponding $\Delta_c = (1 - r)/(1 + r)$ vanishes. In this decoupled limit $\Delta = 0$, the equation separates into position and momentum sectors. The solutions correspond to eigenstates of $x$ and $p$ with eigenvalues $x_0 = p_0 = \sqrt{2E+1}$. These states are non-normalizable, implying a continuous spectrum above the threshold $E_c=-1/2$ and the absence of discrete bound states~\cite{braak_spectral_2023}.
	
	In this regime, the two sectors are completely decoupled. If $[\varphi_1 \ \varphi_2]^{\rm T}$ is an eigenstate, then $[\varphi_1 \ -\varphi_2]^{\rm T}$ is also an eigenstate with opposite parity but the same energy. As a result, the energy gap $\epsilon_{\rm dp}$ between the different parities vanishes identically, and the spectrum is doubly degenerate. 
	
	In contrast, the level spacing within a given parity sector is still governed by the effective harmonic mode with frequency $\omega_{\rm eff}$. Therefore, the gap $\epsilon_{\rm sp}$ within the same parity continues to define the characteristic low-energy scale and fully governs the critical scaling behavior. 
	
	Eliminating $\varphi_1$ yields an effective equation for $\varphi_2$~\cite{chanBoundStatesTwophoton2020}:
	\begin{equation}
		- 2 \partial_x^2 \varphi_2 - \frac{\Delta^2}{4 \left(\frac{x^2}{2} - E -\frac{1}{2}\right)} \varphi_2 = \left( E+\frac{1}{2} \right) \varphi_2.
	\end{equation}
	For bound states ($E < -1/2$), introducing the rescaled variable $x \to \sqrt{2} \kappa x$ with $\kappa^2 = - \left( E + \frac{1}{2} \right) > 0$ allows the equation to be recast as
	\begin{equation}
		- \partial_x^2 \varphi_2 + V \varphi_2 = - \kappa^4 \varphi_2, 
	\end{equation}
	with
	\begin{equation}
		V = - \frac{\Delta^2}{4 \left(x^2 + 1 \right)}.
	\end{equation}
	The effective potential exhibits an inverse-square asymptotic form $V(x) \propto -1/x^2$ as $x \to \infty$, which is known to support an infinite sequence of bound states accumulating toward the continuum threshold in a geometric manner $\sim \lambda^{-n}$~\cite{li_critical_2025}, analogous to the Efimov effect~\cite{zulli_universal_2025}. 
	
	The above analysis provides a microscopic picture of spectral collapse in the isotropic tpQRM. At $\Delta=0$, the collapse originates from the complete loss of confinement, leading to a continuous spectrum above $E_c$. For finite $\Delta$, the inverse-square tail generates an infinite tower of bound states that accumulate toward the same threshold.
	
	Meanwhile, although the gap between different parities vanishes identically in this limit, the gap within the same parity $\epsilon_{\rm sp}$ continues to define the characteristic energy scale, consistent with the main-text identification of the soft mode Eq.~(6). This confirms that the soft mode remains the unique critical excitation, independent of the detailed spectral structure.
	
	\section{Scaling of Observables within the Adiabatic Approximation}
	
	In this section, we show that the critical scaling of all observables, Eqs.~(8-10), (12), and (14) in the main text, is governed by a single energy scale, namely the gap within the same parity $\epsilon_{\rm sp}$. Our goal is to demonstrate that the adiabatic approximation (AA), whose validity has been established in the previous section, provides a controlled framework for deriving these scaling relations.
	
	Within the AA, the approximate eigenstates at $\Delta=\Delta_c$ are
	\begin{equation}
		\ket{\psi_{n,\pm}^{(\rm AA)}} = \frac{1}{\sqrt{2}} \begin{bmatrix}
			S(-\theta) \ket{2n} \\
			\mp (-1)^n S(\theta) \ket{2n}
		\end{bmatrix},
	\end{equation}
	with eigenenergies
	\begin{equation}
		E_{n,\rm c}^{\rm (AA)} = \left( 2n + \frac{1}{2} \right) \beta - \frac{1}{2} + \mathcal{O} \left( \beta^\frac{5}{2} \right).
	\end{equation}
	
	To evaluate observables analytically, it is convenient to express the action of bosonic operators on the ground state in terms of AA eigenstates. Using the identities summarized in Eq.~\eqref{a_relation}, all expectation values can be reduced to overlaps between low-lying states.
	\begin{eqnarray}
		a^2 \ket{\psi_{0}} = a^2 \ket{\psi_{0,-}^{(\rm AA)}}  = \frac{1-\beta}{2\beta} \begin{bmatrix}
			S(-\theta) \ket{2} \\
			- S(\theta) \ket{2}
		\end{bmatrix} - \frac{\sqrt{1-\beta^2}}{2 \sqrt{2} \beta} \begin{bmatrix}
			S(-\theta) \ket{0} \\
			S(\theta) \ket{0}
		\end{bmatrix} = \frac{1-\beta}{\sqrt{2} \beta} \ket{\psi_{1,+}^{(\rm AA)}} - \frac{\sqrt{1-\beta^2}}{2 \beta} \ket{\psi_{0,+}^{(\rm AA)}}, \nonumber \\
		a^{\dagger 2} \ket{\psi_{0}} = a^{\dagger 2} \ket{\psi_{0,-}^{(\rm AA)}} = \frac{1+\beta}{2\beta} \begin{bmatrix}
			S(-\theta) \ket{2} \\
			- S(\theta) \ket{2}
		\end{bmatrix} - \frac{\sqrt{1-\beta^2}}{2 \sqrt{2} \beta} \begin{bmatrix}
			S(-\theta) \ket{0} \\
			S(\theta) \ket{0}
		\end{bmatrix} = \frac{1+\beta}{\sqrt{2} \beta} \ket{\psi_{1,+}^{(\rm AA)}} - \frac{\sqrt{1-\beta^2}}{2 \beta} \ket{\psi_{0,+}^{(\rm AA)}}, \nonumber \\
		a^{\dagger} a \ket{\psi_{0}} = a^{\dagger} a \ket{\psi_{0,-}^{(\rm AA)}} = \frac{1-\beta}{2\sqrt{2} \beta} \begin{bmatrix}
			S(-\theta) \ket{0} \\
			- S(\theta) \ket{0}
		\end{bmatrix} - \frac{\sqrt{1-\beta^2}}{2\beta} \begin{bmatrix}
			S(-\theta) \ket{2} \\
			S(\theta) \ket{2}
		\end{bmatrix} = \frac{1-\beta}{2 \beta} \ket{\psi_{0,-}^{(\rm AA)}} - \frac{\sqrt{1-\beta^2}}{\sqrt{2} \beta} \ket{\psi_{1,-}^{(\rm AA)}}.
		\label{a_relation}
	\end{eqnarray}
	
	We first consider the quadrature fluctuations.
	\begin{eqnarray}
		\Delta x &=& \sqrt{\braket{x^2} - \braket{x}^2} = \sqrt{\braket{a^2 + a^{\dagger 2} + 2a^{\dagger} a + 1}}, \nonumber \\
		\Delta p &=& \sqrt{\braket{p^2} - \braket{p}^2} = \sqrt{\braket{2a^{\dagger} a + 1 - a^2 - a^{\dagger 2}}},
	\end{eqnarray}
	where $\braket{x} = \braket{p} = 0$ in the even photonic number subspace. Using the relations in \eqref{a_relation},
	\begin{eqnarray}
		\bra{\psi_{0}} a^2 \ket{\psi_{0}} = \frac{1-\beta}{\sqrt{2} \beta} \langle \psi_{0,-}^{(\rm AA)} \ket{\psi_{1,+}^{(\rm AA)}} - \frac{\sqrt{1-\beta^2}}{2 \beta} \langle \psi_{0,-}^{(\rm AA)} \ket{\psi_{0,+}^{(\rm AA)}} = 0, \nonumber \\
		\bra{\psi_{0}} a^{\dagger 2} \ket{\psi_{0}} = \frac{1+\beta}{\sqrt{2} \beta} \langle \psi_{0,-}^{(\rm AA)} \ket{\psi_{1,+}^{(\rm AA)}} - \frac{\sqrt{1-\beta^2}}{2 \beta} \langle \psi_{0,-}^{(\rm AA)} \ket{\psi_{0,+}^{(\rm AA)}} = 0, \nonumber \\
		\bra{\psi_{0}} a^{\dagger} a \ket{\psi_{0}} = \frac{1-\beta}{2 \beta} \langle \psi_{0,-}^{(\rm AA)} \ket{\psi_{0,-}^{(\rm AA)}} - \frac{\sqrt{1-\beta^2}}{\sqrt{2} \beta} \langle \psi_{0,-}^{(\rm AA)} \ket{\psi_{1,-}^{(\rm AA)}} = \frac{1-\beta}{2\beta}.
	\end{eqnarray}
	Substituting into the expresstions for $\Delta x$ and $\Delta p$, we immediately obtain
	\begin{equation}
		\Delta x = \Delta p= \sqrt{ \frac{1-\beta}{\beta} + 1} = \beta^{-\frac{1}{2}} \sim \vert g - g_c \vert^{-\nu}, \quad \nu = 1/4.
	\end{equation}
	Combined with $z\nu=1/2$, this yields the dynamical exponent $z=2$, consistent with Eq.~(8) of the main text.
	
	The photon number scales as
	\begin{equation}
		\braket{a^\dagger a} = \frac{1-\beta}{2\beta} \sim |g-g_c|^{-1/2} \sim \epsilon_{\rm sp}^{-1},
	\end{equation}
	reflecting the rapid growth of quantum fluctuations as the bosonic mode softens into a strongly squeezed state, consistent with Eq.~(10) of the main text. Meanwhile, the ground-state order parameter---the atomic polarization---scales as
	\begin{equation}
		\braket{\sigma_x} = - \frac{1}{2} \left[ \bra{0} S(-2\theta) \ket{0} + \bra{0} S(2\theta) \ket{0}\right] = \sqrt{\beta} \sim |g-g_c|^{1/4} \sim \sqrt{\epsilon_{\rm sp}},
	\end{equation}
	vanishing continuously as the qubit evolves from the down state to an equal-weight superposition, as expected for a continuous quantum phase transition and consistent with Eq.~(9) of the main text.
	
	We next consider the quantum Fisher information (QFI), whose spectral representation reads
	\begin{equation}
		F_Q = 4 \sum_{n \neq 0} \frac{\vert \bra{\Phi_n(g)} \partial_g H \ket{\Phi_0 (g)} \vert^2}{\left( E_n(g) - E_0 (g) \right)^2},
	\end{equation}
	where $H \ket{\Phi_n (g)} = E_n(g) \ket{\Phi_n (g)}$ and 
	\begin{equation}
		\partial_g H = \frac{1+r}{2} \sigma_{z} \left( a^2 + a^{\dagger 2} \right)  + \frac{1-r}{2} i \sigma_y \left( a^2 - a^{\dagger 2} \right).
	\end{equation} 
	Parity symmetry enforces $[\Pi, \partial_g H]$ since
	\begin{equation}
		\Pi \partial_g H \Pi^{-1} = \frac{1+r}{2} (-\sigma_{z}) \left( (ia)^2 + (-ia^{\dagger})^2 \right)  + \frac{1-r}{2} (-i \sigma_y) \left( (ia)^2 - (-ia^{\dagger})^2 \right) = \partial_g H,
	\end{equation}
	thus for a non-degenerate ground state, $\bra{\psi_{0,-}^{(\rm AA)}} \partial_g H \ket{\psi_{n,+}^{(\rm AA)}}$ must vanish, restricting the sum to states within the same parity. As a result, the dominant contribution arises from the lowest excitation, yielding	
	\begin{equation} 
		F_Q \simeq 4 \frac{\vert \bra{\psi_{1,-}^{(\rm AA)}} \partial_g H \ket{\psi_{0,-}^{(\rm AA)}} \vert^2}{\left( E_{1,\rm c}^{\rm (AA)} - E_{0,\rm c}^{\rm (AA)} \right)^2} = \frac{\vert \bra{\psi_{1,-}^{(\rm AA)}} (1+r) \sigma_{z} \left( a^2 + a^{\dagger 2} \right)  + (1-r) i \sigma_y \left( a^2 - a^{\dagger 2} \right) \ket{\psi_{0,-}^{(\rm AA)}} \vert^2}{(2\beta)^2}
	\end{equation} 
	Using relations \eqref{a_relation}, we have
	\begin{eqnarray}
		F_Q &\simeq& \frac{\left \vert \bra{\psi_{1,-}^{(\rm AA)}} [(1+r) \sigma_{z} + (1-r) i \sigma_y] \frac{1-\beta}{\sqrt{2} \beta} \ket{\psi_{1,+}^{(\rm AA)}}  + \bra{\psi_{1,-}^{(\rm AA)}} [(1+r) \sigma_{z} - (1-r) i \sigma_y] \frac{1+\beta}{\sqrt{2} \beta} \ket{\psi_{1,+}^{(\rm AA)}} \right \vert^2}{(2\beta)^2} \nonumber \\
		&=& \frac{\left \vert \bra{\psi_{1,-}^{(\rm AA)}}(1+r) \sigma_{z} \frac{\sqrt{2}}{\beta} \ket{\psi_{1,+}^{(\rm AA)}}  - \bra{\psi_{1,-}^{(\rm AA)}} \sqrt{2}(1-r) i \sigma_y \ket{\psi_{1,+}^{(\rm AA)}} \right \vert^2}{(2\beta)^2} \simeq \frac{(1+r)^2}{2\beta^4} \nonumber \\
		&\sim& |g-g_c|^{-2} \sim \epsilon_{\rm sp}^{-4},
	\end{eqnarray}
	which gives Eq.~(12) of the main text. This corresponds to the strongest algebraic divergence allowed for pure states in Hermitian systems and highlights the extreme sensitivity of QFI near criticality.
	
	Taken together, all observables exhibit scaling governed by $\epsilon_{\rm sp}$,
	\begin{equation}
		\Delta x, \Delta p \sim \epsilon_{\rm sp}^{-1/2}, \quad
		\braket{a^\dagger a} \sim \epsilon_{\rm sp}^{-1}, \quad
		\braket{\sigma_x} \sim \epsilon_{\rm sp}^{1/2}, \quad
		F_Q \sim \epsilon_{\rm sp}^{-4}.
	\end{equation}
	These results demonstrate that the anisotropic tpQRM belongs to the same universality class as the standard QRM~\cite{ashhab_superradiance_2013, hwang_quantum_2015}. The emergent soft mode thus provides the unique mechanism controlling both static observables and metrological response.
	
	\section{Kibble-Zurek Scaling of the Residual Energy}
	
	In this section, we derive the scaling of the residual energy, Eq.~(14) of the main text, under a slow quench follow the procedure in Ref.~\cite{hwang_quantum_2015} and show that the nonequilibrium dynamics are governed by the same soft-mode gap $\epsilon_{\rm sp}$ that controls the equilibrium critical behavior. Our goal is to demonstrate that the Kibble-Zurek (KZ) scaling emerges directly from the soft-mode structure established in the previous sections.
	
	We consider a linear quench protocol $g(t) = g_f t / \tau_q = \dot{g} t$ where $g_f$ is the final coupling strength and $\dot{g} \ll 1$. At $\Delta = \Delta_c$ and near the critical point, the wavefunction can be expanded in the AA basis,
	\begin{equation}
		\ket{\Psi(t)} = \sum f_{n,\pm}(t) e^{-i \Theta_{n,\pm}(t)} \ket{\psi_{n,\pm}^{(\rm AA)}(t)},
	\end{equation}
	with $\Theta_{n,\pm}(t)=\int_0^t E_{n,\pm}^{(\rm AA)}(t') dt'$.
	The Schr\"{o}dinger equation yields
	\begin{equation}
		\dot{f}_{n,\pm} (t) = - \sum f_{m,\pm} (t) \bra{\psi_{n,\pm}^{\rm (AA)} (g(t))} \partial_{g} \ket{\psi_{m,\pm}^{(\rm AA)} (g(t))} e^{i \left[\Theta_{n,\pm}(t) - \Theta_{m,\pm}(t)\right]}.
	\end{equation}
	Changing variables to $g = \dot{g} t$ gives
	\begin{equation}
		f_{n,\pm}(g) = - \sum \int_{0}^{g} f_{m,\pm} (g') \bra{\psi_{n,\pm}^{\rm (AA)} (g')} \partial_{g'} \ket{\psi_{m,\pm}^{(\rm AA)} (g')} e^{i \left[\Theta_{n,\pm}(g') - \Theta_{m,\pm}(g')\right]} \mathrm{d} g'.
	\end{equation}
	
	Assuming the system is initially prepared in the ground state, $f_{0,-}(0)=1$, adiabatic perturbation theory~\cite{dziarmaga_dynamics_2010} yields
	\begin{equation}
		f_{n,\pm}(g) \simeq - \int_{0}^{g} \bra{\psi_{n,\pm}^{\rm (AA)} (g')} \partial_{g'} \ket{\psi_{0,-}^{(\rm AA)} (g')} e^{i \left[\Theta_{n,\pm}(g') - \Theta_{0,-}(g')\right]} \mathrm{d} g'.
	\end{equation}
	Evaluating the rapidly oscillating integral using integration by parts,
	\begin{equation}
		\int_{x_1}^{x_2} f(x) e^{i A g(x)} \mathrm{d}x = \left. \frac{f(x)}{iA g(x)}e^{i A g(x)} \right\vert_{x_1}^{x_2} + \mathcal{O}(A^{-2}), 
	\end{equation}
	yields
	\begin{eqnarray}
		f_{n,\pm}(g) &\simeq& \left. i\dot{g} \frac{\bra{\psi_{n,\pm}^{(\rm AA)} (g) \ket{\partial_{g}} \psi_{0,-}^{(\rm AA)} (g)}}{E_{n,\pm}^{(\rm AA)} (g) - E_{0,-}^{(\rm AA)} (g)} e^{i \left[\Theta_{n,\pm}(g) - \Theta_{0,-}(g)\right]} \right \vert_0^g + \mathcal{O} (\dot{g}^2) \nonumber \\
		&\simeq& - i\dot{g} \frac{\sqrt{2}(1+r)}{8\beta^3} e^{i \left[\Theta_{n,\pm}(g) - \Theta_{0,-}(g) \right]} \delta_{n,1} \delta_{\pm,-}.
	\end{eqnarray}
	
	Due to parity symmetry, only transitions within the same parity sector are allowed, and the dominant contribution arises from the lowest excitation. To leading order,
	\begin{equation}
		f_{1,-}(g) \simeq - i\dot{g} \frac{\sqrt{2} (1+r)}{8 (1-g^2/g_c^2)^{3 z\nu} } e^{i \left[\Theta_{1,-}(g) - \Theta_{0,-}(g) \right]}.
	\end{equation}
	
	The residual energy at the end of the quench is
	\begin{equation}
		E_r(g_f) \simeq \epsilon_{\rm sp} \vert f_{1,-}(g_f) \vert^2
		\simeq \tau_q^{-2} \frac{g_f^2 / g_c^2}{16 (1 - g_f^2 / g_c^2)^{5 z\nu}}.		
	\end{equation}
	Thus, for quenches ending far from the critical point, this reduces to the adiabatic scaling $E_r \sim \tau_q^{-2}$.
	
	As the system approaches the critical point, the vanishing gap leads to a breakdown of adiabaticity. Within the KZ framework~\cite{kibble_topology_1976, zurek_cosmological_1985}, this occurs when the intrinsic relaxation time $\tau_{\rm rel} \sim \epsilon_{\rm sp}^{-1}$ becomes comparable to the driving time scale $\tau_{\rm drive} \sim |\dot{\epsilon}_{\rm sp}/\epsilon_{\rm sp}|^{-1}$. Solving this condition near the critical point yields the freeze-out scale 
	\begin{eqnarray}
		4 \left( 1- \frac{g_K^2}{g_c^2} \right)^{2z\nu} = 2 \frac{g_K g_f}{\tau_q} (1+r)^2 \left( 1- \frac{g_K^2}{g_c^2} \right)^{-z\nu} \nonumber \\
		\left( 1-g_K/g_c \right)^{3 z\nu} = \frac{g_K g_f}{2 \tau_q} (1+r)^2 \left( 1 + g_K/g_c \right)^{-3 z\nu}.
	\end{eqnarray}
	
	Evaluating the freeze-out condition at $g_f = g_c$ and $g_K \to g_c$, one obtains 
	\begin{eqnarray}
		1 - g_K/g_c &\simeq& \left( \frac{2^{-3 z\nu}}{2\tau_q} \right)^\frac{1}{3 z\nu} = \left( \frac{2^{-3 z\nu - 1}}{\tau_q} \right)^\frac{1}{3 z\nu}
		\nonumber \\
		g_K / g_c &\simeq& 1 - (4\sqrt{2} \tau_q)^{- \frac{1}{3 z\nu}}.
	\end{eqnarray}
	Substituting $g_K$ into the expression for the residual energy gives
	\begin{equation}
		E_r \simeq \tau_q^{-2} \frac{g_K^2 / g_c^2}{16 (1 - g_K^2 / g_c^2)^{5 z\nu}} 
		\simeq \tau_q^{-2} \frac{(4\sqrt{2} \tau_q)^{\frac{5}{3}}}{16} 
		\propto \tau_q^{-\frac{1}{3}},
	\end{equation}
	which is the Eq.~(14) of the main text. For $z\nu = 1/2$, this yields
	\begin{equation}
		E_r \sim \tau_q^{-\frac{z\nu}{z\nu + 1}},
	\end{equation}
	in agreement with the universal KZ scaling.
	
	The above results demonstrate that the nonequilibrium dynamics are entirely controlled by the soft-mode gap $\epsilon_{\rm sp}$. In particular, the same exponent $z\nu$ governs both equilibrium scaling,
	\begin{equation}
		\epsilon_{\rm sp} \sim |g-g_c|^{z\nu},
	\end{equation}
	and nonequilibrium KZ dynamics,
	\begin{equation}
		E_r \sim \tau_q^{-\frac{z\nu}{1+z\nu}}.
	\end{equation}
	
	This establishes a direct correspondence between excitation-gap scaling and quench dynamics. The anisotropic tpQRM therefore belongs to a dynamical universality class entirely governed by a single critical mode, with nonequilibrium scaling inherited from the equilibrium soft-mode physics.
	
	\bibliography{refs}
	
\end{document}
